# Supplementary material for: Unraveling the Structure of Ultracold Mesoscopic Molecular Ions
Source: arXiv:1703.02812 ancillary file (2017-06-09)
Supplement: Supplementary file 1 [file supplementary.pdf]

# Supplemental Material for "Unraveling the Structure of Ultracold Mesoscopic Molecular Ions"


J. M. Schurer,[1,2,*] A. Negretti,[1,2] and P. Schmelcher[1,2,†]

[1] *Zentrum für Optische Quantentechnologien, Universität Hamburg, Luruper Chaussee 149, 22761 Hamburg, Germany*

[2] *The Hamburg Centre for Ultrafast Imaging, Universität Hamburg, Luruper Chaussee 149, 22761 Hamburg, Germany*



(Dated: June 8, 2017)



This supplementary material for the letter "Unraveling the Structure of Ultracold Mesoscopic Molecular Ions" includes details on the atom-ion interaction, the frame transformations, the employed model approaches, and the effective force analysis. A discussion of the ab-initio ML-MCTDHB approach and the convergence of the numerical results is also presented.


## HAMILTONIAN

For completeness, let us give the Hamiltonian scaled into the units of the atom-ion interaction potential $R^*$ and $E^*$

$$\hat{H}/E^* = \frac{\mu}{m_\mathrm{I}}\left(-\frac{\partial^2}{\partial z_\mathrm{I}^2} + \frac{z_\mathrm{I}^2}{\tilde{l}_\mathrm{I}^4}\right) + \frac{\mu}{m_\mathrm{A}}\sum_{i=1}^{N}\left(-\frac{\partial^2}{\partial z_i^2} + \frac{z_i^2}{\tilde{l}_\mathrm{A}^4}\right) + \tilde{g}\sum_{i<j=1}^{N}\delta(z_i - z_j) + \sum_{i=1}^{N} V_\mathrm{AI}(z_i - z_\mathrm{I}). \tag{S1}$$

with the reduced mass $\mu = m_\mathrm{A} m_\mathrm{I}/(m_\mathrm{A} + m_\mathrm{I})$, the trap length scales $\tilde{l}_{\mathrm{A,I}} = \sqrt{\hbar/(m_{\mathrm{A,I}}\omega_{\mathrm{A,I}})}/R^*$ and the scaled atom-ion interaction $\tilde{g} = g/(R^* E^*)$ for the most general case of unequal trap frequencies $\omega_\mathrm{A}$ and $\omega_\mathrm{I}$ and masses $m_\mathrm{A}$ and $m_\mathrm{I}$ for the atoms and the ion, respectively.

## MODEL POTENTIAL FOR THE ATOM-ION INTERACTION

In one spatial dimension, the interaction between an atom and an ion scales with the relative coordinate $z$ like $-1/z^4$. However, this is only the behavior for large distances. In case $z$ becomes smaller than a certain cutoff distance, the interaction starts to deviate from this power law behavior [1]. Therefore, we use a model for the atom-ion interaction defined in Ref. [2] as:

$$V_\mathrm{AI}(z) = \mathrm{v}_0 e^{-\gamma z^2} - \frac{1}{z^4 + 1/\kappa}, \tag{S2}$$

scaled in units of $R^*$ and $E^*$, which is very well-suited for our many-body investigations. The specific choice of the model potential, i.e. for the values of $\mathrm{v}_0$, $\gamma$, and $\kappa$, parametrizes the short-range behavior [2]. The latter determines the scattering length as well as the energy of the bound states. In this work, we use $\mathrm{v}_0 = 250$, $\kappa = 80$ , and $\gamma = 4\sqrt{10\kappa}$. We refer the interested reader to Ref. [2] for further details.

## FRAME TRANSFORMATIONS

In order to obtain a numerically efficient description of the hybrid atom-ion system (see below), we employed a frame transformation from the laboratory frame (LF) to the ion frame (IF) coordinates and alternatively from the LF to the center of mass frame (CMF). Here we provide the reader with the coordinate transformation as well as the transformed Hamiltonians.

*Ion Frame.–* The IF coordinates and their momenta are given by $Z_\mathrm{I} = z_\mathrm{I}$, $Z_i = z_i - z_\mathrm{I}$ and $\partial_{z_\mathrm{I}} = \partial_{Z_\mathrm{I}} - \sum_i^N \partial_{Z_i}$, $\partial_{z_i} = \partial_{Z_i}$, respectively. By applying this transformation to the Hamiltonian (1), we obtain, in units of $R^*$ and $E^*$,

the Hamiltonian:

$$H = -\frac{\mu}{m_{\rm I}}\left(\frac{\partial}{\partial Z_{\rm I}} - \sum_i^N \frac{\partial}{\partial Z_i}\right)^2 - \frac{\mu}{m_{\rm A}}\sum_{i=1}^N \frac{\partial^2}{\partial Z_i^2} + \frac{\mu}{m_{\rm A}\tilde{l}_{\rm A}^4}\sum_{i=1}^N (Z_i + Z_{\rm I})^2 + \frac{\mu}{m_{\rm I}\tilde{l}_{\rm I}^4} Z_{\rm I}^2$$
$$+ \tilde{g}\sum_{i<j=1}^N \delta(Z_i - Z_j) + \sum_{i=1}^N V_{\rm AI}(Z_i). \tag{S3}$$

with $\tilde{g} = g/(R^* E^*)$ and $\tilde{l}_{\rm A,I} = l_{\rm A,I}/R^*$. Now we can compute the ground state of $H$ using ML-MCTDHB resulting in a wave function given in IF coordinates. Hence, in order to investigate for example densities in the LF, we have to make the inverse transformation of this wave function. Since this is computationally very expensive due to the high dimensionality of the wave function, we transform only the reduced quantities of interest. To this end, we define the reduced density matrices for the ion $\hat{\rho}_{\rm I} = {\rm Tr}_N\left[|\psi\rangle\langle\psi|\right]$ and the atoms $\hat{\rho}_{\rm A}^m = {\rm Tr}_{{\rm I},N-m}\left[|\psi\rangle\langle\psi|\right]$, where ${\rm Tr}_N$ (${\rm Tr}_{{\rm I},N-m}$) indicates the trace over all $N$ atoms (the ion and $N-m$ atoms). The eigenvalues and eigenvectors of $\hat{\rho}_{\rm A}^1$ ($\hat{\rho}_{\rm I}$) in spectral representation are the natural populations $\lambda_i^{\rm A(I)}$ and natural orbitals $|\Phi_i^{\rm A(I)}\rangle$, respectively. Taking the density matrix $\hat{\rho} = |\psi\rangle\langle\psi|$ in the LF and in the IF coordinates:

$$\begin{aligned} \text{LF:} \quad & \rho_{LF}(z_{\rm I}, z_1, \cdots, z_N, z_{\rm I}', z_1', \cdots, z_N') \\ \text{IF:} \quad & \rho_{IF}(Z_{\rm I}, Z_1, \cdots, Z_N, Z_{\rm I}', Z_1', \cdots, Z_N'). \end{aligned}$$

and using the transformation to the IF, we can relate the density (matrix)[3] in both frames traced over one atom:

$$\begin{aligned} \rho_{IF}^{N-1}(Z_{\rm I}, Z_1, \cdots, Z_{N-1}, Z_{\rm I}, Z_1', \cdots, Z_{N-1}') \equiv & \int {\rm d}Z_N \rho_{IF}(Z_{\rm I}, Z_1, \cdots, Z_N, Z_{\rm I}, Z_1', \cdots, Z_N) \\ = & \int {\rm d}Z_N \rho_{LF}(Z_{\rm I}, Z_1 + Z_{\rm I}, \cdots, Z_N + Z_{\rm I}, Z_{\rm I}, Z_1' + Z_{\rm I}, \cdots, Z_{N-1}' + Z_{\rm I}, Z_N + Z_{\rm I}) \\ = & \int {\rm d}z_N \rho_{LF}(Z_{\rm I}, Z_1 + Z_{\rm I}, \cdots, z_N, Z_{\rm I}, Z_1' + Z_{\rm I}, \cdots, Z_{N-1}' + Z_{\rm I}, z_N) \\ \equiv & \rho_{LF}^{N-1}(Z_{\rm I}, Z_1 + Z_{\rm I}, \cdots, Z_{N-1} + Z_{\rm I}, Z_{\rm I}, Z_1' + Z_{\rm I}, \cdots, Z_{N-1}' + Z_{\rm I}). \end{aligned}$$

Repeating this procedure $N-2$ times, we find the transformation rule for the reduced atom-ion density matrix

$$\rho_{IF}^1(Z_{\rm I}, Z_1, Z_{\rm I}, Z_1') = \rho_{LF}^1(Z_{\rm I}, Z_1 + Z_{\rm I}, Z_{\rm I}, Z_1' + Z_{\rm I}) \tag{S4}$$

leading to the conclusion that the ionic density $\rho_{\rm I}$ is in both frames equal

$$\rho_{\rm IF}^0(Z_{\rm I}) = \rho_{\rm LF}^0(Z_{\rm I}), \qquad \rho_{\rm IF}^0(z_{\rm I}) = \rho_{\rm LF}^0(z_{\rm I}), \tag{S5}$$

and that the transformation of the atomic density matrix to the LF is given by

$$\rho_{\rm A}^1(z_1, z_1') = \int {\rm d}z_{\rm I} \rho_{IF}^1(z_{\rm I}, z_1 - z_{\rm I}, z_{\rm I}, z_1' - z_{\rm I}). \tag{S6}$$

*Center of Mass Frame.–* In case the trapping frequencies coincide $\omega = \omega_{\rm A} = \omega_{\rm I}$, the center of mass motion decouples from the relative coordinates. We choose the transformation $R = \left(m_{\rm I} z_{\rm I} + m_{\rm A}\sum_{i=1}^N z_i\right)/M$ and $r_i = z_i - z_{\rm I}$ with the momenta $\partial_R = \partial_{z_{\rm I}} + \sum_i^N \partial_{z_i}$ and $\partial_{r_i} = \partial_{z_i} - \frac{m_{\rm A}}{M}\partial_R$. and the total mass $M = m_{\rm I} + N m_{\rm A}$. Application of this transformation to the Hamiltonian (1) leads in units of $R^*$ and $E^*$ to

$$H = H_R - \sum_i^N \frac{\partial^2}{\partial r_i^2} - \frac{2\mu}{m_{\rm I}}\sum_{i<j}^N \frac{\partial}{\partial r_i}\frac{\partial}{\partial r_j} + \frac{1}{\tilde{l}_r^4}\sum_i^N r_i^2 + \frac{2}{\tilde{l}_r^4}\sum_{i<j}^N r_i r_j + \tilde{g}\sum_{i<j=1}^N \delta(r_i - r_j) + \sum_{i=1}^N V_{\rm AI}(r_i), \tag{S7}$$

with the center of mass part

$$H_R = -\frac{\mu}{M}\frac{\partial^2}{\partial R^2} + \frac{\mu}{M\tilde{l}_R^4} R^2 \tag{S8}$$

containing the harmonic oscillator length of the center of mass motion $\tilde{l}_R = \sqrt{\hbar/(M\omega)}/R^*$, the relative motion $\tilde{l}_r = \sqrt{\hbar/(\mu\omega_r)}/R^*$, and the frequency $\omega_r = \sqrt{\frac{m_\mathrm{A}}{\mu}\left(1 - \frac{m_\mathrm{A}}{M}\right)}\omega$. Importantly, we can write the total wave function in the CMF as a product

$$\psi(R, r_1, \cdots, r_N) = \psi_R(R)\psi_r(r_1, \cdots, r_N). \tag{S9}$$

Hence the problem reduces to $N$ interacting trapped bosons. For the ground state, we can write the center of mass wave function as a Gaussian

$$\psi_R(R) = \left(\frac{1}{\pi l_R^2}\right)^{1/4} \exp\left[-\frac{R^2}{2l_R^2}\right] \tag{S10}$$

of width

$$\langle R^2\rangle = \sigma_R^2 = \frac{m_\mathrm{I}}{M}\sigma_0^2. \tag{S11}$$

The reduced density matrix in the CMF is given by $\hat{\rho}_\mathrm{A}^\mathrm{CMF} = \mathrm{Tr}_{N-1}\left[|\psi_r\rangle\langle\psi_r|\right]$ and has eigenvalues $\lambda_i^\mathrm{CMF}$ and eigenvectors $|\Phi_i^\mathrm{CMF}\rangle$, respectively. There are no simple relations between the reduced quantities of the CMF and the ones of the other two frames. This means that the coordinate transformation can only be applied to the full $(N+1)$-dimensional wave function and not to the corresponding reduced quantities, which limits its practical use to very few particles. As a consequence, this restricts the possible analysis which can be accurately performed from calculations in the CMF. Below, we sketch, however, how such limitations can be tackled for specific situations in case one transforming to the IF.

## WAVE FUNCTION ANSATZ CLASSES

For both ansatz wave functions [Eq. (2) and Eq. (3)], one can deduce the variational optimal equations of motion for the involved single particle functions $\varphi$ and $\chi$

$$i\partial_t\varphi(x,t) = \left[h_\mathrm{I} + N\langle\chi|h_{1\mathrm{I}}|\chi\rangle\right]\varphi(x,t) \tag{S12}$$
$$i\partial_t\chi(y,t) = \left[h_1 + \langle\varphi|h_{1\mathrm{I}}|\varphi\rangle + (N-1)\langle\chi|h_{12}|\chi\rangle\right]\chi(y,t) \tag{S13}$$

with $x = z_\mathrm{I}$ ($Z_\mathrm{I}$) and $y = z_1$ ($Z_1$) for the MF (Gross) ansatz. Also the contained operators are different due to the frame transformation.

| Mean-field | Gross | |
|---|---|---|
| $h_\mathrm{I}^\mathrm{MF} = -\frac{\mu}{m_\mathrm{I}}\partial_{z_\mathrm{I}}^2 + V_\mathrm{I}(z_\mathrm{I})$ | $h_\mathrm{I}^\mathrm{G} = -\frac{\mu}{m_\mathrm{I}}\partial_{Z_\mathrm{I}}^2 + V_\mathrm{I}(Z_\mathrm{I})$ | (S14) |
| $h_1^\mathrm{MF} = -\frac{\mu}{m_\mathrm{A}}\partial_{z_1}^2 + V_\mathrm{A}(z_1)$ | $h_1^\mathrm{G} = -\partial_{Z_1}^2 + V_\mathrm{AI}(Z_1)$ | (S15) |
| $h_{1\mathrm{I}}^\mathrm{MF} = V_\mathrm{AI}(z_\mathrm{I} - z_1)$ | $h_{1\mathrm{I}}^\mathrm{G} = V_\mathrm{A}(Z_\mathrm{I} + Z_1) + \frac{2\mu}{m_\mathrm{I}}\partial_{Z_\mathrm{I}}\partial_{Z_1}$ | (S16) |
| $h_{12}^\mathrm{MF} = V_{AA}(z_1 - z_2)$ | $h_{12}^\mathrm{G} = V_{AA}(Z_1 - Z_2) - \frac{2\mu}{m_\mathrm{I}}\partial_{Z_1}\partial_{Z_2}$ | (S17) |

Note that we use $\langle\chi|\hat{O}|\chi\rangle$ and $\langle\varphi|\hat{O}|\varphi\rangle$ as a short-hand notion for the partial trace over the operator $\hat{O}$ with respect to the atomic ($z_1$ or $Z_1$) and the ionic ($z_\mathrm{I}$ or $Z_\mathrm{I}$) coordinate, respectively.

*The Gross ansatz.–* For the ground state, equation Eq. (S12) in the Gross frame simplifies due to symmetry ($\langle\chi|\partial_{Z_1}|\chi\rangle = \langle\chi|Z_1|\chi\rangle = 0$) to a single particle of mass $m_\mathrm{I}$ in a harmonic trap. However, the trap is given by the sum of the ion trap and all atom traps $[V_\mathrm{I}(Z_\mathrm{I}) + NV_\mathrm{A}(Z_\mathrm{I})]$, resulting in the trap frequency

$$\omega_{MF} = \sqrt{\left[1 + N\frac{m_\mathrm{I} l_\mathrm{I}^4}{m_\mathrm{A} l_\mathrm{A}^4}\right]} \tag{S18}$$

and hence the width for the ionic density given by

$$\sigma_{\mathrm{I,MF}}^2 = \frac{\omega_\mathrm{I}}{\omega_{MF}}\sigma_0^2 \tag{S19}$$

scaling with $1/\sqrt{N+1}$.

## SIMPLE MODELS

In the main text, we use two simple models to describe our numerical data: i) the center of mass localization of a molecule with fixed bound state; ii) the Thomas-Fermi model. These, we describe in some detail here.

*Trapped Molecule.–* A molecule in a trap experiences mainly a localization of the center of mass coordinate as long as the width of the bound state (or binding length) is smaller than the confinement length $\sigma_0$. Employing Hamiltonian (S7) and omitting coupling terms between the relative coordinates $r_i$, one can assume the relative wave function $\psi_r(r_1, \cdots, r_N)$ to be a product such that the total wave function is given by $\psi(R, r_1, \cdots, r_N) = \psi_R(R) \prod_i^N \chi_0(r_i)$ with $\chi_0$ being the bound state of the atom-ion potential. With this ansatz, we can derive the width of the ionic and the atomic density distribution to be:

$$\sigma_{\mathrm{I,M}}^2 = \sigma_R^2 + \left(\frac{m_{\mathrm{A}}}{M}\right)^2 N\sigma_r^2, \tag{S20}$$

$$\sigma_{\mathrm{A,M}}^2 = \sigma_R^2 + \left[\left(\frac{m_{\mathrm{A}}}{M}\right)^2 (N-1) + \left(\frac{m_{\mathrm{A}}}{M} - 1\right)^2\right] \sigma_r^2, \tag{S21}$$

with the bound state width $\sigma_r^2 = \int r^2 |\chi_0(r)|^2 \mathrm{d}r$ and the center of mass variance $\sigma_R^2$ given in Eq. (S11). Equations (S20) and (S21) provide a simple estimate for the ionic as well as the atomic density variance. They are valid as long as the interactions between the atoms are weak, thus in particular for $g = 0$.

*Molecule in a Thomas-Fermi cloud.–* For $N_{\mathrm{TF}}$ bosons in a harmonic trap, the density profile of the atoms can be described in the high density limit by the so-called Thomas-Fermi density profile

$$\rho_{\mathrm{TF}}(z) = \frac{\mu_{\mathrm{TF}} - \frac{\mu z^2}{m_{\mathrm{A}} l_{\mathrm{A}}^4}}{g} \tag{S22}$$

with the chemical potential $\mu_{TF} = [\frac{3gN_{\mathrm{TF}}}{4}\sqrt{\mu/(m_{\mathrm{A}} l_{\mathrm{A}}^4)}]^{2/3}$. In our system, only those atoms which are not bound to the ion contribute to the build-up of such a density, thus $N_{\mathrm{TF}} = N - N_c$. Therefore, for large $N$, we can estimate that the total atomic density variance behaves like the sum of the width of the TF gas with $N_{\mathrm{TF}}$ atoms plus the width of the molecule at the critical particle number $N_c$:

$$\sigma_{\mathrm{A,TF}}^2(N_{\mathrm{TF}}) = \frac{1}{N}\sigma_{TF}^2(N_{\mathrm{TF}}) + \frac{N_c}{N}\sigma_{\mathrm{A}}^2(N = N_c) \tag{S23}$$

with the Thomas-Fermi variance $\sigma_{\mathrm{TF}}^2 = \int_{-z_{\mathrm{TF}}}^{z_{\mathrm{TF}}} z^2 \rho_{TF}(z) \mathrm{d}z$ and the Thomas-Fermi radius $z_{\mathrm{TF}}$ defined by $\rho_{\mathrm{TF}}(z_{\mathrm{TF}}) = 0$. One can easily find that $\sigma_{\mathrm{TF}}^2/N \propto (N - N_c)^{5/3}/N$.

## EFFECTIVE FORCE ANALYSIS

Inspired by Refs. [4, 5], we can make use of the knowledge of the complete many-body wave function in order to derive explicitly the effective force acting on the ion in the IF. By this, we can determine the effective potential for the ion. The force acting on the ion in the IF can be found via the Heisenberg equation of motion $\hat{F}_{\mathrm{I}} = \partial_t \hat{p}_{\mathrm{I}} = -[\partial_{Z_{\mathrm{I}}}, \hat{H}]$. Computing the expectation value for a general wave function of our hybrid system, we obtain

$$\langle \hat{F}_{\mathrm{I}} \rangle^{\mathrm{IF}} = \int \mathrm{d}Z_{\mathrm{I}} \rho_{\mathrm{I}}(Z_{\mathrm{I}}) F_{\mathrm{I}}^*(Z_{\mathrm{I}}) \tag{S24}$$

where

$$F_{\mathrm{I}}^*(Z_{\mathrm{I}}) = F_{\mathrm{I}}^0(Z_{\mathrm{I}}) + \Delta F_{\mathrm{I}}(Z_{\mathrm{I}}) \tag{S25}$$

is the effective force to which the ion in the IF is exposed. It consists of a mean-field contribution stemming from a harmonic confinement of frequency (S18),

$$F_{\mathrm{I}}^0 = -\left(\frac{2\mu}{m_{\mathrm{I}} l_{\mathrm{I}}^4} + \frac{2\mu N}{m_{\mathrm{A}} l_{\mathrm{A}}^4}\right) Z_{\mathrm{I}}, \tag{S26}$$

and an additional force resulting from correlations beyond the ansatz (3)

$$\Delta F_{\rm I}(Z_{\rm I}) = -\frac{1}{\rho_{\rm I}(Z_{\rm I})}\int {\rm d}Z_1\cdots {\rm d}Z_N\left(\frac{2\mu}{m_{\rm A}\tilde{l}_{\rm A}^4}\sum_i Z_i\right)\rho(Z_{\rm I}, Z_1,\cdots,Z_N). \tag{S27}$$

We emphasize that the above definition of an effective force enables us to compute the local force, which gives interesting insights.

The introduction of an effective single particle of mass $m^*$ in a trap of frequency $\omega^*$, as done in the main text, assumes a force on the ion given by $F_{\rm I}^*(Z_{\rm I}) = -2\mu/(m^* l^{*4})Z_{\rm I}$ with $l^*/l_{\rm I} = \sqrt{m_{\rm I}\omega_{\rm I}/(m^*\omega^*)}$. Hence, the force $\Delta F_{\rm I}$ has to be (approximatively) linear in $Z_{\rm I}$

$$\Delta F_{\rm I} \approx -2BZ_{\rm I} \tag{S28}$$

with $B = -\frac{1}{2}\partial_{Z_{\rm I}}\Delta F_{\rm I}|_{Z_{\rm I}=0}$. For an induced trapping force, we expect $B > 0$, while for an anti-trapping force, $B < 0$. Indeed, the resulting value for $B$ shown in Supp. Fig. 1 is negative for all investigated parameters. Using $B$ and the ionic width $l^* = \sqrt{2}\sigma_{\rm I}$ , we can derive the effective mass and the effective trap frequency via

$$\frac{m^*}{m_{\rm I}} = \left(\frac{l_{\rm I}}{l^*}\right)^4\left(1 + N\frac{m_{\rm I}l_{\rm I}^4}{m_{\rm A}\tilde{l}_{\rm A}^4} + B\frac{l_{\rm I}^4 m_{\rm I}}{\mu}\right)^{-1} \tag{S29}$$

and

$$\frac{\omega^*}{\omega_{\rm I}} = \frac{m_{\rm I}l_{\rm I}^2}{(m^* l^{*2})}, \tag{S30}$$

respectively. Let us emphasize here that the introduction of this effective single particle is justified by the observation that the ionic density distribution is Gaussian which goes hand-in-hand with a linear force. In order to test this assumption, we derive the variance of the ionic density distribution additionally via the central density $\rho_{\rm I}(0)$ and the fourth moment $\langle Z_{\rm I}^4\rangle$. For a Gaussian distribution, these should be connected via $\sigma_{\rm I}^2 = 1/(\rho_{\rm I}(0)^2 2\pi)$ and $\sigma_{\rm I}^2 = \sqrt{\langle Z_{\rm I}^4\rangle/3}$. In Supp. Fig. 1, we see good agreement between these expression, except for $g = 3E^*R^*$ and large $N$. In this regime, the effective particle description breaks down which corresponds to the case $g = 3E^*R^*$ and $N > 16$ in the main text.

Now let us explicate the way how the factor $B$ is derived from IF and CMF calculations. Starting with a wave function given in the IF, we see that we can execute $N-1$ integrals in Eq. (S27) due to the bosonic exchange symmetry. Hence, we obtain

$$\Delta F_{\rm I}(Z_{\rm I}) = -\frac{N}{\rho_{\rm I}(Z_{\rm I})}\int {\rm d}Z\rho_{\rm IF}^1(Z, Z_{\rm I})\left(\frac{2\mu}{m_{\rm A}\tilde{l}_{\rm A}^4}Z\right). \tag{S31}$$

Interestingly, one observes that for a wave function of class (3), the additional force on the ion vanishes ($B = 0$), since $\rho_{\rm IF}^1(Z, Z_{\rm I}) = \rho_{\rm A}^1(Z)\rho_{\rm I}(Z_{\rm I})$[6]. Therefore, the fact that $B \neq 0$, that is, the existence of an induced additional trapping potential for the ion due to the atoms, results from correlations between atoms and ion in the IF which could not be captured by the mean-field ansatz (3). The derivation of $B$ from the CMF data is comparatively difficult, since we need to employ a coordinate transformation to the IF before executing the integrals. Hence, $\Delta F_{\rm I}$ is given by

$$\Delta F_{\rm I}(Z_{\rm I}) = -\frac{1}{\rho_{\rm IF}^0(Z_{\rm I})}\int {\rm d}Z_1\cdots {\rm d}Z_N\left(\frac{2\mu}{m_{\rm A}\tilde{l}_{\rm A}^4}\sum_j Z_j\right)|\psi_R(Z_{\rm I} + \frac{m_{\rm A}}{M}\sum_i Z_i)|^2|\psi_r(Z_1,\cdots,Z_N)|^2. \tag{S32}$$

resulting in the following expression for $B$

$$B = \frac{-2\mu}{m_{\rm I}l_{\rm I}^6}\left(\frac{m_{\rm A}}{m_{\rm I}}\right)^2\sqrt{\frac{M}{m_{\rm I}}}\left(\frac{l^*}{l_{\rm I}}\right)\int {\rm d}Z_1\cdots {\rm d}Z_N\left(\sum_i Z_i\right)^2 e^{-\frac{m_{\rm A}^2}{m_{\rm I}Ml_{\rm I}^2}(\sum_i Z_i)^2}|\psi_r(Z_1,\cdots,Z_N)|^2. \tag{S33}$$

Such an expression can be evaluated in the spirit of an expectation value $\langle\psi_r|(\sum_i \hat{Z}_i)^2\hat{O}_{\rm exp}|\psi_r\rangle$ with the operator $\hat{O}_{\rm exp}$ representing the exponential. Here one first applies $\hat{O}_{\rm exp}$ by exploiting the analogy to the time evolution operator and executing a temporal evolution with MCTDHB and the non-hermitian Hamiltonian $\hat{H}_{exp} = \hbar/i\frac{m_{\rm A}^2}{m_{\rm I}Ml_{\rm I}^2}(\sum_i \hat{Z}_i)^2$, second applies the operator $(\sum_i \hat{Z}_i)^2$, and third computes the overlap. The result for $B$ given in Supp. Fig. 1.

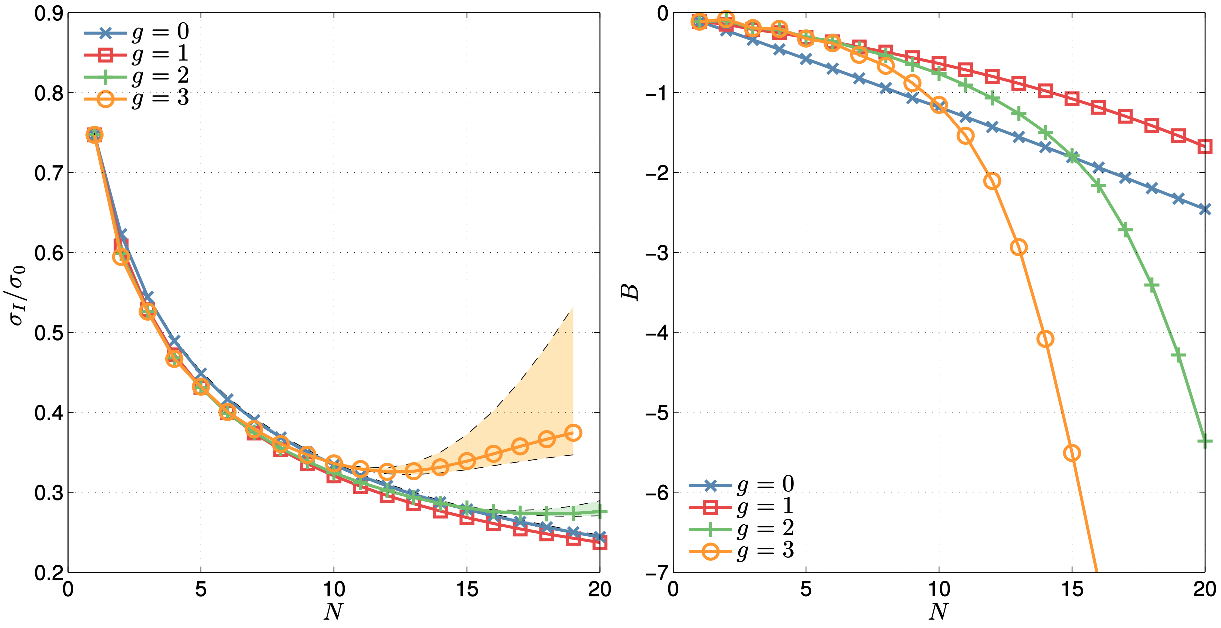


SUPP. FIG. 1. (Left) Quality of the assumption of a Gaussian ion density distribution: The variance of the ionic density distribution (solid lines) together with the latter derived via the central density (upper dashed line) and via the fourth moment (lower dashed lines) (see text)for $g/(E^*R^*) = 0, 1, 2, 3$ (cross, square, plus, circle). (Right) Calculated additional force prefactor $B$ as a function of $N$ in the IF for $g/(E^*R^*) = 0, 1, 2, 3$ (cross, square, plus, circle).

## COMPUTATIONAL METHOD AND CONVERGENCE

In the multi-layer multi-configuration time-dependent Hartree method for bosons, the total wave function is expanded as a product of $M$ time-dependent orthonormal wave functions for the ion and the atoms $|\Psi\rangle = \sum_{ij}^{M} A_{ij}(t)|\Psi_i^{\mathrm{A}}(t)\rangle|\Psi_j^{\mathrm{I}}(t)\rangle$. The wave functions for the atoms are expressed in numberstates $|\Psi_i^{\mathrm{A}}\rangle = \sum_{\mathbf{n}|N} C_{\mathbf{n}}^{i}(t)|\mathbf{n}\rangle_t$, which are build by *time-dependent* single-particle functions $\{\psi_k(t)\}_{k=1}^{m}$, where the vector $\mathbf{n} = (n_1, n_2, \cdots)$ contains the occupations $n_j$ of the $j$-th single-particle function. We emphasize that here not only the coefficients $A_{ij}$ but also the single particle functions $\psi_k$ are chosen variationally optimal in time, allowing for a very efficient representation of the wave function. The values for $m$ and $M$ specify the degree of approximation. In oder to judge whether these are large enough, one commonly investigates the natural population of the ionic $\hat{\rho}_{\mathrm{I}}$ and the atomic $\hat{\rho}_{\mathrm{A}}^{1}$ density matrix. In the following, we discuss the quality of the employed truncation. Thereby, we focus on the most challenging situation discussed in the main text, namely for the highest atomic interaction $g = 3E^*R^*$.

The description of a many-body wave function as a sum of products of functions of the individual LF coordinates becomes inefficient in case bound states are present. Hence, we have chosen the IF and the CMF (see definitions above), for the above-given ML-MCTDHB expansion scheme. In the IF, already the simple product state ansatz (3) can give reasonable approximations for small $N$ and small $g$, even though such an ansatz is not exact already for $N = 1$ due to the coupling terms in Eq. (S3). For small $N$, the latter cause population of the second bound state (see main text). In simulations with $M = 4$ and $m = 5$, the highest observed natural population of the least populated natural orbital of $\hat{\rho}_{\mathrm{I}}$ is on the order of $\lambda_m^{\mathrm{I}} \approx 10^{-5}$ and for $\hat{\rho}_{\mathrm{A}}^{1}$ on the order of $\lambda_m^{\mathrm{A}} \approx 10^{-3}$ (see Supp. Fig. 2), which can be considered to be converged. Moreover, each natural population only changes marginally when comparing the simulations with $m = 4$ and $m = 5$. A second, only recently proposed [7], convergence test is the comparison of the center-of-mass variance of the ML-MCTDHB solution to the analytical expectation. We find that as long as all atoms are bound to the ion, i.e., $N < N_c$, the center-of-mass variance is reproduced and approaches the corresponding analytic curve. However, for $N > N_c$, larger deviations become visible. Hence, we would slightly overestimate [see Eq.(S20)] the variance of the ion [8] in computations in the IF. Therefore, in order to further test and improve our results, in particular the calculations of the variances, we resort to the CMF coordinate system defined above. For the special case $\omega_{\mathrm{A}} = \omega_{\mathrm{I}}$, the Hamiltonian exactly separates into a center of mass and a relative part, i.e. $M_{\mathrm{CMF}} = 1$ such that the relative problem can be viewed as a system of $N$ interacting bosonic atoms which can be solved with an MCTDHB ansatz. In this way, we can avoid the error in the center of mass variance present in the IF. Since also here the natural populations of the least occupied natural orbital of the reduced density matrix in the CMF is on the

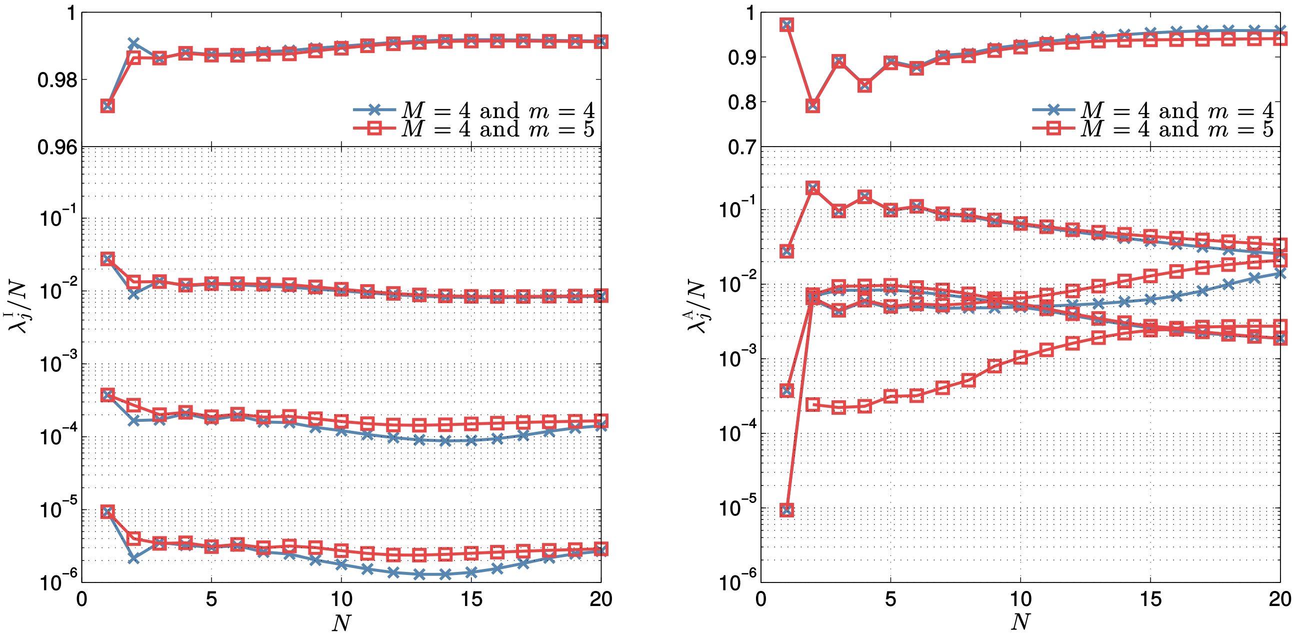


SUPP. FIG. 2. Natural populations in the IF of the ionic density matrix $\mathrm{Tr}_N\,[\rho_{IF}]$ (left) and of the one-body reduced density matrix of the atoms $\mathrm{Tr}_{\mathrm{I},N-1}\,[\rho_{IF}]$ (right) as a function of $N$ for $g/(R^*E^*) = 3$ and $m = 4, 5$ (cross,square). Note that the natural populations of the ionic density matrix are equal to the natural population of the atomic density matrix $\mathrm{Tr}_{\mathrm{I}}\,[\rho_{IF}]$, as a consequence of the Schmidt decomposition for bipartite systems. Further, notice that the $\lambda_i^{\mathrm{A(I)}}$ are by definition ordered such that $\lambda_1^{\mathrm{A(I)}} > \lambda_2^{\mathrm{A(I)}} > \cdots \lambda_m^{\mathrm{A(I)}}$ and that the $y$-axis has a linear and a logarithmic part to enhance visibility.

order of $\lambda_m^{\mathrm{CMF}} \approx 10^{-3}$ for $m_{\mathrm{CMF}} = 5$, we have further strong evidence that the results shown in the main text are indeed converged. For completeness, we provide an additional test of the convergence of the total energy. This is done by comparing the relative differences of the total energies obtained for two configurations $a = (M, m)$ ($a = (m_{\mathrm{CMF}})$) and $b = (M, m)$ ($b = (m_{\mathrm{CMF}})$)

$$\nu = \frac{E_a - E_b}{E_b}. \tag{S34}$$

In Supp. Fig. 3, we see that the single orbital simulations show strong deviations to the four orbital version for both the IF and the CMF (blue and yellow lines). In contrast, the relative difference between the respective four and five orbital computations (green and dashed brown line) is only a few percent. Moreover, the relative difference between the five orbital simulations of the IF and the CMF (pink line) are of similar size.


* jschurer@physnet.uni-hamburg.de
† pschmelc@physnet.uni-hamburg.de



[1] Z. Idziaszek, T. Calarco, and P. Zoller, Phys. Rev. A **76**, 033409 (2007).
[2] J. M. Schurer, P. Schmelcher, and A. Negretti, Phys. Rev. A **90**, 033601 (2014).
[3] Note that we have to use $Z_{\mathrm{I}} = Z'_{\mathrm{I}}$.
[4] G. Astrakharchik and L. Pitaevskii, Phys. Rev. A **70**, 013608 (2004).
[5] J. Bonart and L. F. Cugliandolo, EPL (Europhysics Letters) **101**, 16003 (2013).
[6] Further, it is assumed that $\rho_{\mathrm{A}}(Z)$ is symmetric.
[7] J. G. Cosme, C. Weiss, and J. Brand, Phys. Rev. A **94**, 043603 (2016).
[8] The impact on the atomic variance is less severe.

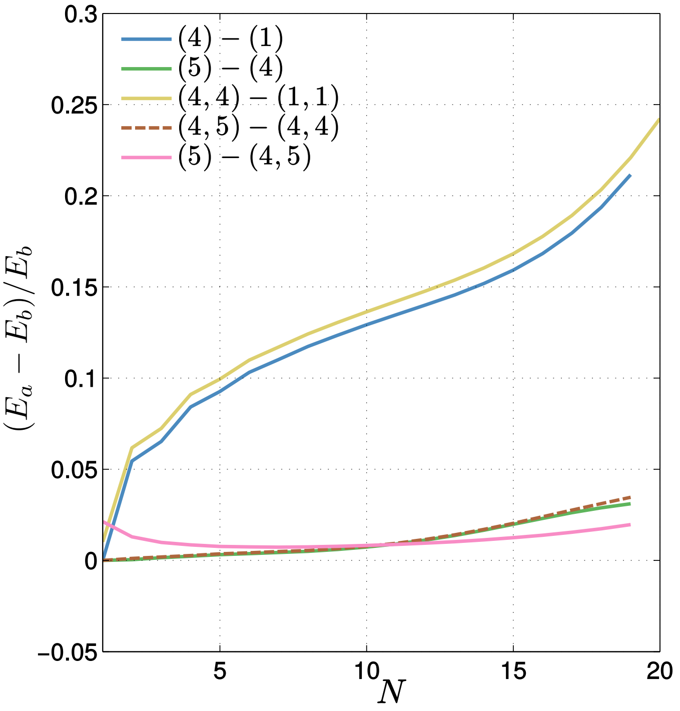


SUPP. FIG. 3. Relative differences $(E_a - E_b)/E_b$ of the total energy for different ML-MCTDHB expansions $a$ and $b$. In the figure legend, the number of used orbitals for configuration $a$ and $b$ are given. A single number $(m_{\mathrm{CMF}})$ indicates a computation in the CMF while two numbers point to an expansion in the IF with $(M, m)$.
